# Supplementary material for: Index analysis: an approach to understand signal transduction with application to the EGFR signalling pathway
Source: arXiv:2302.08815 source file (2023-02-17)
Supplement: Supplementary file 1 [file Knoechel_etal_2023_IndexAnalysis_Supplement.pdf]

# Supplementary Material

## Index analysis: an approach to understand signal transduction with application to the EGFR signalling pathway

Jane Knöchel, Charlotte Kloft, Wilhelm Huisinga

### S1 EGFR system

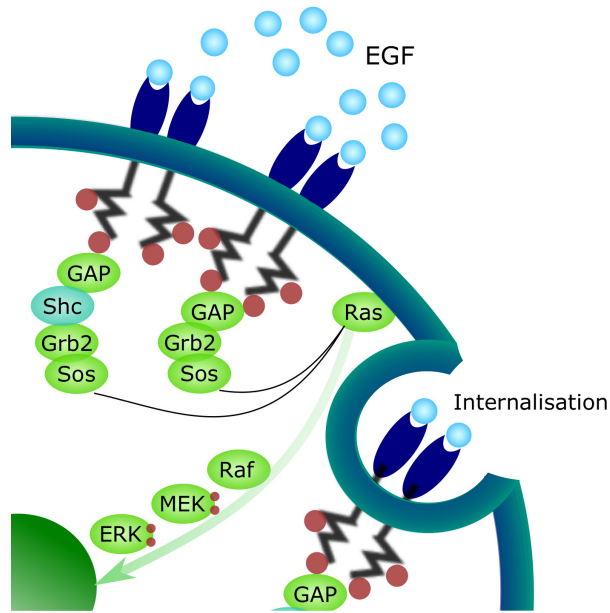

**Figure S1.** Simplified illustration of EGFR signalling cascade.

The EGFR signalling network is activated by the binding of the ligand EGF to its receptor (EGFR) and results in a transient double-phosphorylation of the extracellular signal-regulated kinase (ERK-PP); see Figure S1.

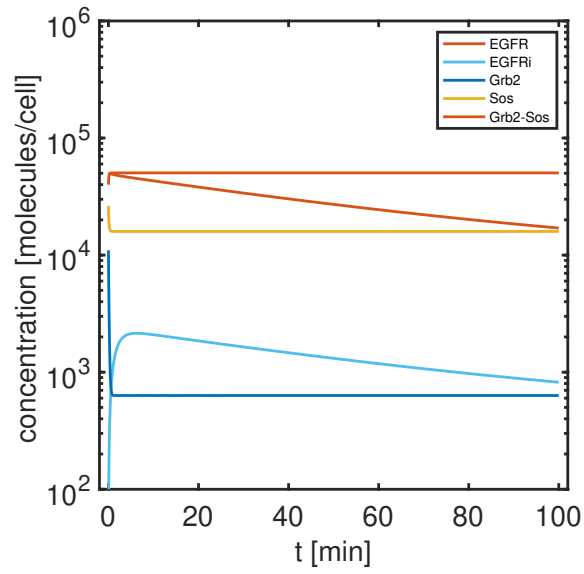

**Figure S2. EGFR signalling network prior to a stimulus.** An illustration of state variables that are not in steady state prior to any EGF stimulus. For details on the model, see Material Section in the main article.

## S2 Computation ir-indices

The input-response index for a single input state variable and a single output state variable is real-valued and can be written in terms of two local sensitivity coefficients

$$\text{ir}_k(t^*) = \left( \frac{1}{T} \int_{t^*}^T \mathcal{S}_{r,k}(t, t^*)^2 dt \right)^{\frac{1}{2}} \cdot |\mathcal{S}_{k,i}(t^*, t_0)| \quad (\text{S1})$$

with sensitivity coefficients

$$\mathcal{S}_{m,j}(t_2, t_1) = [\mathcal{S}(t_2, t_1)]_{m,j} = \left[ \frac{\partial \Phi^{t_2, t_1} x}{\partial x} \Big|_{x=x_{\text{ref}}(t_1)} \right]_{m,j}. \quad (\text{S2})$$

To compute the ir-indices in eq. (S1) numerically, we solved an extended system of ODEs to determine  $\mathcal{S}(t_2, t_1)$  in eq. (S2):

$$\frac{d}{dt}x(t) = f(x(t); p) \quad (\text{S3})$$

$$\frac{d}{dt}\mathcal{S}(t, t_1) = \frac{\partial f(x(t); p)}{\partial x} \cdot \mathcal{S}(t, t_1) \quad (\text{S4})$$

on  $t \in [t_1, t_2]$  with initial conditions  $x(t_1) = x_{\text{ref}}(t_1)$  and  $\mathcal{S}(t_1, t_1) = \text{Id}$ . See, e.g., [1, 3.1] for details.

## S3 Extension to time-dependent input or fixed output time

We defined sensitivity based input-response indices for the special case of an impulse input (i.e., activation of the signalling network at the initial time). The extension to time-dependent inputs  $u(\cdot)$  is easily possible. In this case, the system equations often take the form

$$\frac{dx}{dt}(t) = f(x(t); p) + g(x(t)) \cdot u(t)$$

with an appropriately defined function  $g$ .

For an impulse input and time-dependent output the controllability and observability indices are defined as

$$\mathcal{O}_k(t^*) = \left( \frac{1}{T} \int_{t^*}^T \mathcal{S}_{r,k}(t, t^*)^2 dt \right)^{\frac{1}{2}} \quad \text{and} \quad c_k(t^*) = \mathcal{S}_{k,i}(t^*, t_0). \quad (\text{S5})$$

In the case of a time-dependent input, both,  $\mathcal{O}_k(t^*)$  and  $c_k(t^*)$  in eq. (S5) would be defined as integrated quantities, while the identity  $\text{ir}_k(t^*) = \mathcal{O}_k(t^*)c_k(t^*)$  continues to hold. Vice versa, if the output is a quantity of interest at a specific time point, the integral part of the input-response index in eq. (S1) could be replaced by a sensitivity at the specific output time point.

## S4 Additional index analysis for small-scale illustrative model systems

### S4.1 Index analysis for parallel pathway model

Considered the following simple parallel pathway reaction model sketched in Figure S3. In the model, the signal A activates S into B and C, which in turn activate D. Furthermore, B and C may be deactivated to S again. In this example, A is considered the input and D the response variable. We study two different scenarios given by the parameters in Table S1.

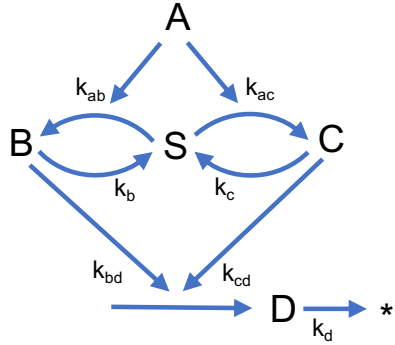

**Figure S3.** Reaction network of the parallel pathways model.

**Table S1. Model specification for the parallel pathway model.** For the two scenarios of the model in Figure S3, the parameter values are stated below. The time span was  $t \in [0, 0.05]$  min, the input A, and the response D. The initial conditions were  $(A_0, B_0, C_0, D_0) = (20, 0, 0, 0)$  nM, in addition to  $S_0$  (in nM) specified below. Units:  $k_{ab}, k_{ac}, k_{bd}, k_{cd}$  in 1/nM/min; all other reaction rate constants in 1/min.

| Scenario       | $S_0$ | $k_{ab}$ | $k_{ac}$ | $k_b$ | $k_c$ | $k_{bd}$ | $k_{cd}$ | $k_d$ |
|----------------|-------|----------|----------|-------|-------|----------|----------|-------|
| no crosstalk   | 3000  | 50/300   | 1/300    | 5     | 500   | 0.4      | 11       | 25    |
| with crosstalk | 10    | 50       | 1        | 5     | 500   | 0.4      | 11       | 25    |

Figure S4A shows the time course of the state variables, while Figure S4B shows the normalised ir-indices. The dynamic importance of state variables changes substantially during the first 0.01 min: While the input A quickly falls below the threshold, S and B substantially increase and then decrease still within the first 0.01 min. During the same time, the response D steadily increases. Only the state variable C stays far below the threshold of 10%. Consequently, we would consider all state variables except C as dynamically important.

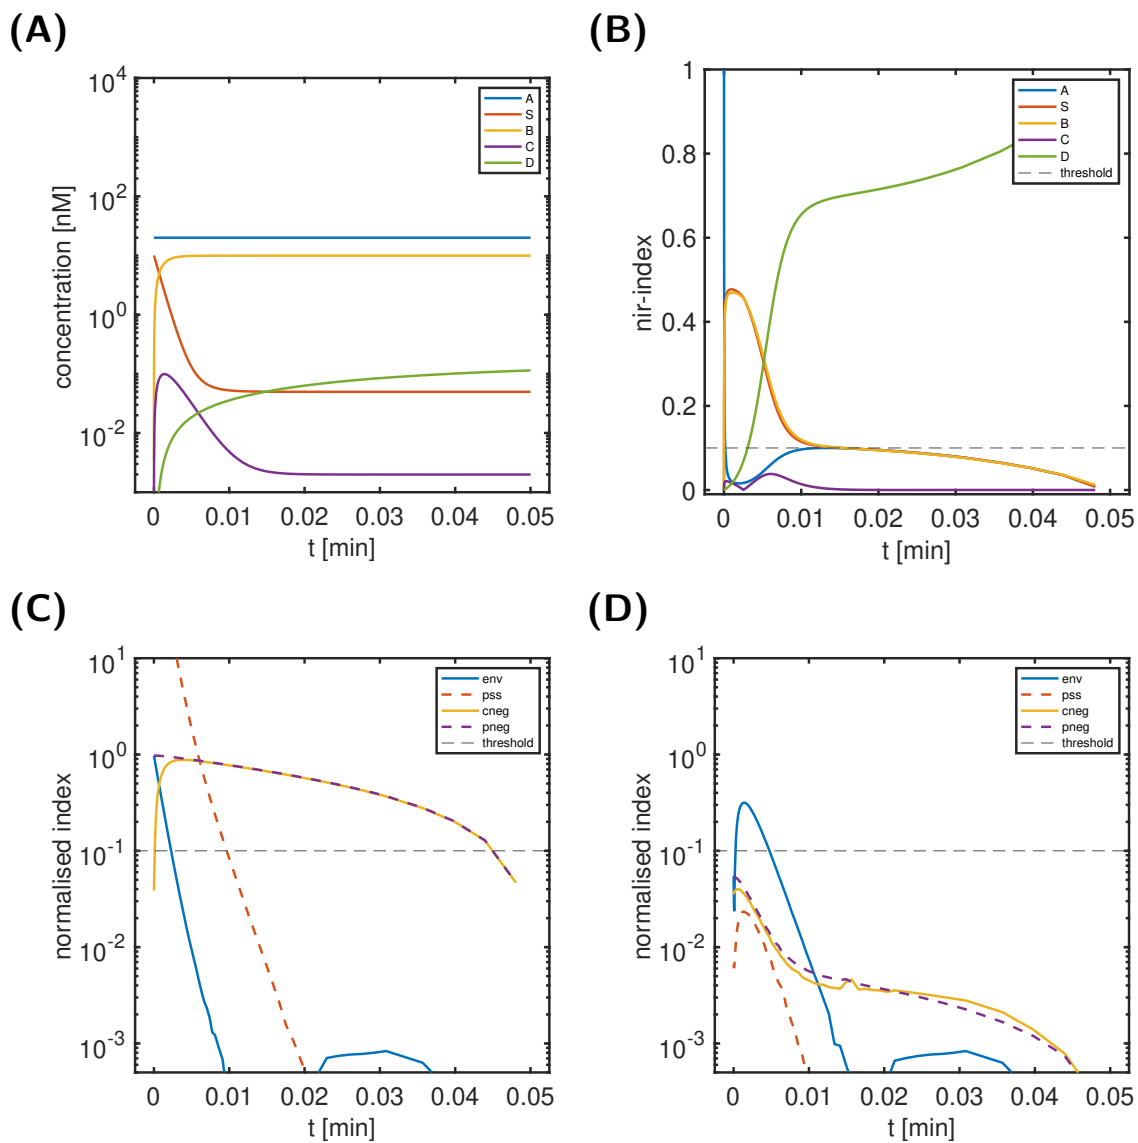

**Figure S4. Scenario 'with crosstalk' of the parallel pathways model: time course of state variables and normalised indices.** A: Time course of state variables and B: normalized ir-indices. C: State classification indices for states B and D: for C.

The bottom graphics of Figure S4 show the state classification indices for two states, B (C) and C (D). Again, a state classification index below the threshold is considered indicative of the corresponding index classification type (environmental, in partial steady state, negligible). From the normalised ir-index we would expect for B none of the state-classification indices below the threshold. This is indeed the case, as shown in the Figure S4C. Figure S4D gives further insight on the potential nature of the state C. All but the env-index are below the threshold.

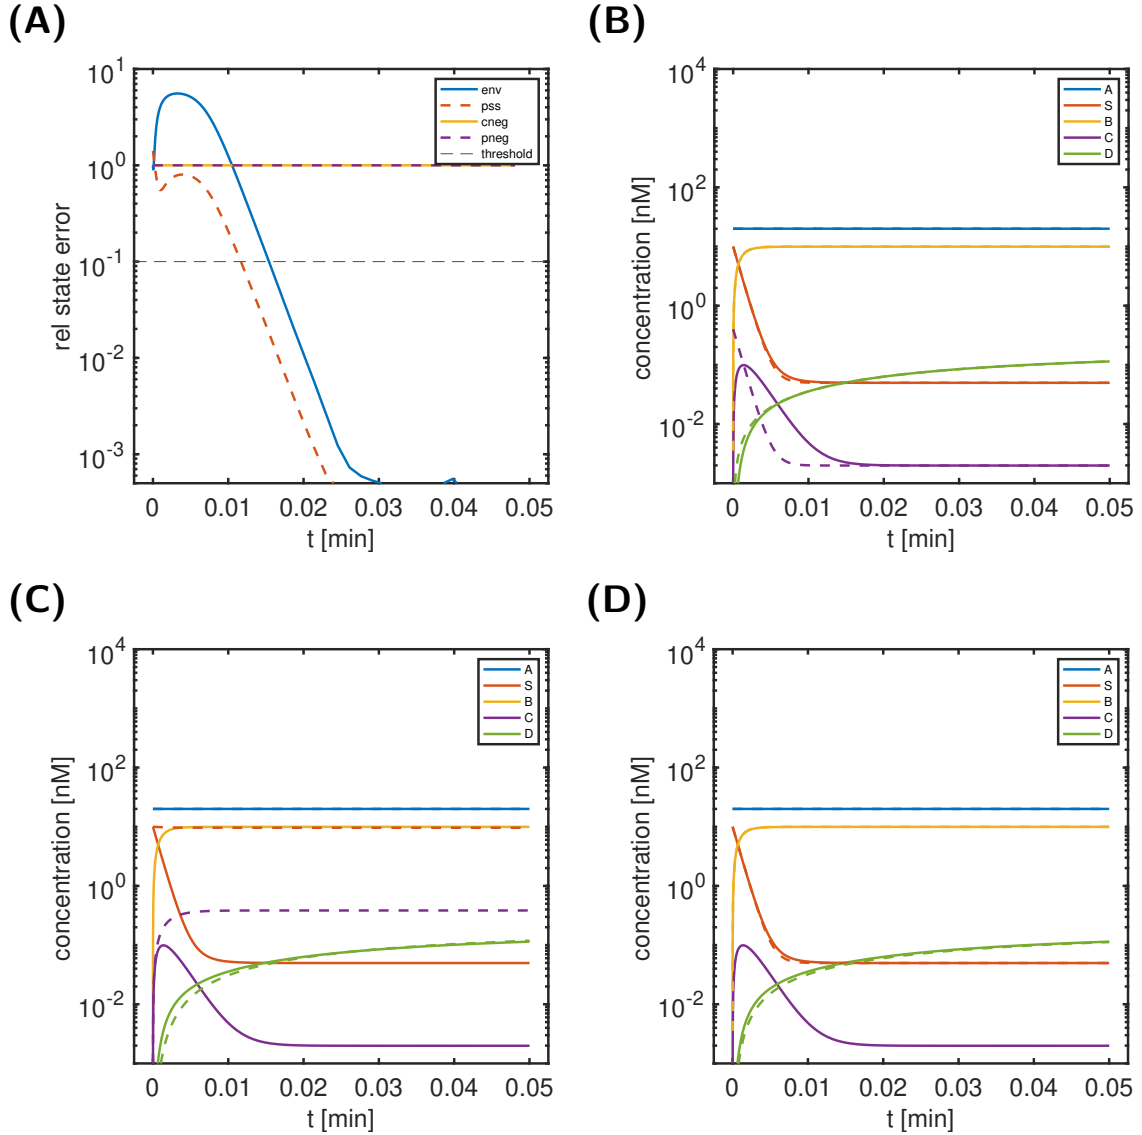

**Figure S5. Scenario 'with crosstalk' of the parallel pathways model: Relative state approximation error and modified dynamics.** A: Relative state approximation errors for C. B: Comparison of reference dynamics (solid lines) and modified dynamics from  $t^* = 0$  (dashed lines) for C in partial steady state or D: completely neglected. C: Comparison of reference dynamics (solid lines) and modified dynamics from  $t^* = 0$  (dashed lines) for B completely neglected.

For a final classification of C, also the relative state approximation error (shown in Figure S5) is taken into account. However, none of the relative state approximation errors is constantly below the threshold. Hence, C is neither classified as environmental nor in partial steady state. To illustrate the latter, Figure S5B shows the reference solution and the solution of the modified system (dashed lines) with C in partial steady state. While the approximation error for the output looks reasonable (as we would expect from the state classification index), the approximation error for the state itself is substantial (as we would expect from the relative state approximation error, Figure S5A: the red dashed line at  $t = 0$  is even above  $10^0$ ).

Finally, we analysed the impact of completely neglecting one of the two pathways, i.e., B or C. From the

normalised ir-indices (Fig. S4C&D), we infer that for both, B and C, the cneg-index at  $t = 0$  is below the threshold. Therefore, we would expect an acceptable approximation of the reduced model with B or C completely neglected (from time  $t = 0$  on). Figure S5C&D shows the reference solution and the solution of the modified system (dashed lines) with B (left) or C (right) completely neglected. The impact on the response D is in both cases small—in line with the normalised ir-index at  $t = 0$  (Fig. S4C&D). Looking at the normalised cneg-index (solid yellow line) of the entire time span, however, we see a marked difference between the two state variables: While for C, the cneg-index is below the threshold for the entire time span, for B it is only below the threshold at the very beginning and at the very end. If we would evolve the reference system up to, e.g., time  $t = 0.01$  and only then completely neglect B, we would see a relatively large error in the response variable (yellow line almost  $10^0$ ), while doing the same for C, we would see almost no error in the response variable (yellow line even below  $10^{-2}$ ). This is an important difference! The fact that the cneg-index for B is only low initially indicates that the system is capable of compensating for a complete loss of B, if it happens from the onset of the signal, while at later times, it is not able to compensate without a marked impact on the response D. In contrast, the system is able to compensate for a loss of C at any time, from signal onset at  $t = 0$  to the very end.

In the above scenario, the crosstalk is caused by the competition for the limited resource of S. Due to the specific parameter values, S is much more strongly activated to B than to C. As a consequence, C can be completely neglected with only minor impact on the response. If, however, B is missing, then C is able to activate D with a very similar profile. This feature disappears, if there is no resource limitation of S, i.e., no crosstalk: Figures S6A&B shows the concentration-time profiles and the normalised ir-indices.

Figures S6C&D shows the state classification indices for B (left) and C (right). In contrast to the scenario with crosstalk, for B also the cneg index is close to 1 initially. Hence, completely neglecting B from  $t = 0$  should have a large impact on the response. This can be seen from Figure S7A, which shows the reference solution and the solution of the modified system (dashed lines) with B completely neglected. Hence, C is not able to activate D in a similar manner as B does, if the latter is missing. The impact of lacking C, however, does not change quantitatively between the scenarios with/without crosstalk, as can be inferred from Figure S6D, and Figure S7B.

Finally, from bottom panel of Figure S7, we conclude that S can be considered as environmental, since considering S being constant does have only negligible impact on the response (bottom left, blue line) as well as on the state itself (bottom right, blue line). This is in line with our expectation, since the presence or absence of crosstalk is linked to S being a limited or abundant resource, respectively (see also  $S_0$  in Table S1).

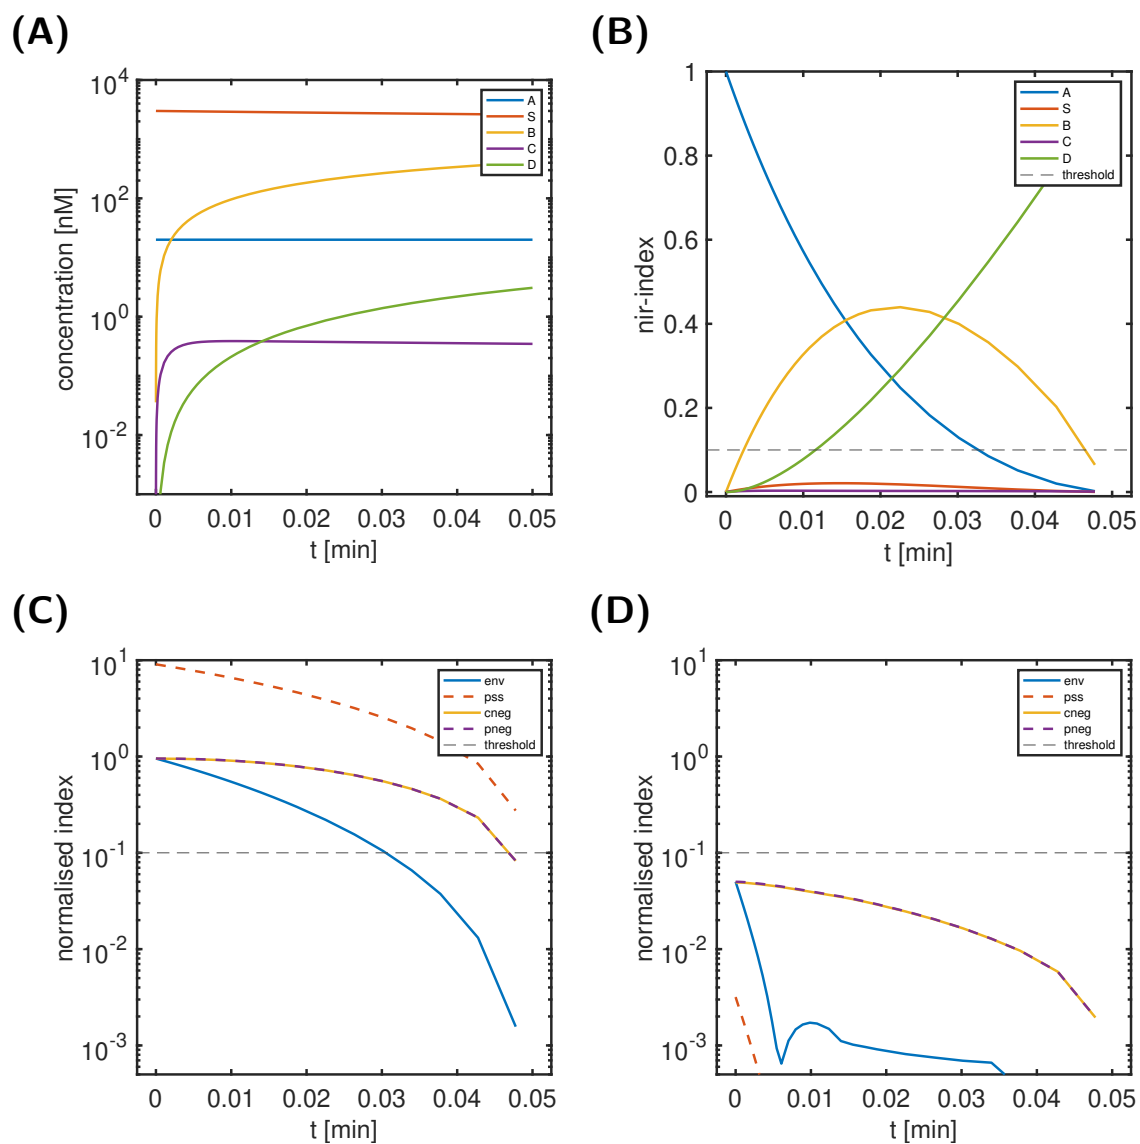

**Figure S6. Scenario no crosstalk of the parallel-pathways model:** A: Time course of state variables and B: normalised ir-indices. C: state classification indices for B and D: for C.

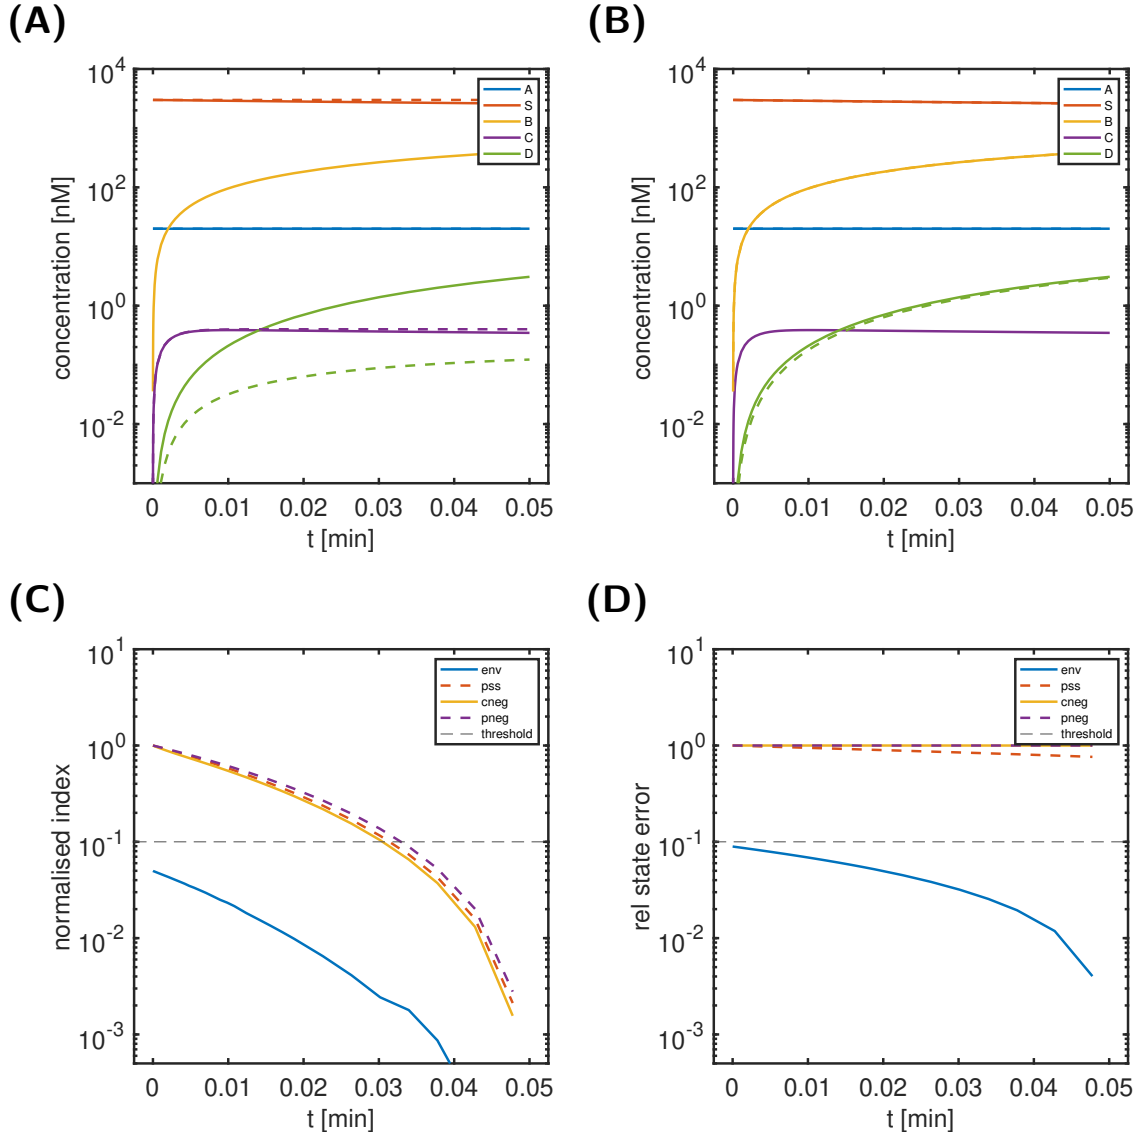

**Figure S7. Scenario no crosstalk of the parallel-pathways model:** A: Comparison of reference dynamics (solid lines) and modified dynamics from  $t^* = 0$  (dashed lines) for B and B: for C being completely neglected. C: state classification indices and D: relative state approximation errors for  $S$ .

## S4.2 Index analysis for enzyme substrate model

Considered the simple enzyme kinetics model sketched in Figure S8. In the model, the protein A is transformed into substrate S, which subsequently forms a complex C with an enzyme E. The complex either dissociates or is catabolised to a product P. In this example, A is considered the input and P the response variable. We study two different scenarios given by the parameters in Table S2. The parameters sets were chosen to illustrate the application to this well-known example and indicate extensions to account for conservation laws.

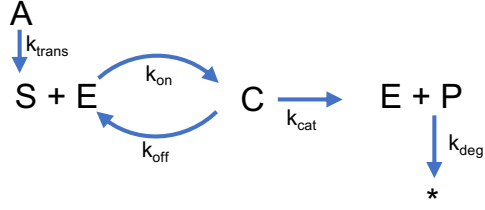

**Figure S8.** Reaction network of the enzyme kinetics model.

**Table S2. Model specification for the enzyme kinetics model.** For the two scenarios of the model in Figure S8, the parameter values are stated below. The time span was  $t \in [0, 30]$  min, the input A, and the response P. The initial conditions were  $(A_0, S_0, C_0, P_0) = (50, 0, 0, 0)$  nM, in addition to  $E_0$  (in nM) specified below. Units:  $k_{\text{on}}$  in 1/nM/min; all other reaction rate constants in 1/min.

| Scenario | $E_0$ | $k_{\text{on}}$ | $k_{\text{off}}$ | $k_{\text{cat}}$ | $k_{\text{trans}}$ |
|----------|-------|-----------------|------------------|------------------|--------------------|
| 1        | 25    | 1               | 900              | 5                | 0.5                |
| 2        | 2     | 0.2             | 10               | 1                | 0.1                |

Figure S9A&B shows the time course of the state variables (left) and the normalised ir-indices (right). Except for E and C, all state variables are at some point in time above the threshold and are thus classified as dynamically importance. Figure S9C&D depicts the state classification indices for C and E. We hypothesise that C is in partial steady state and E is environmental.

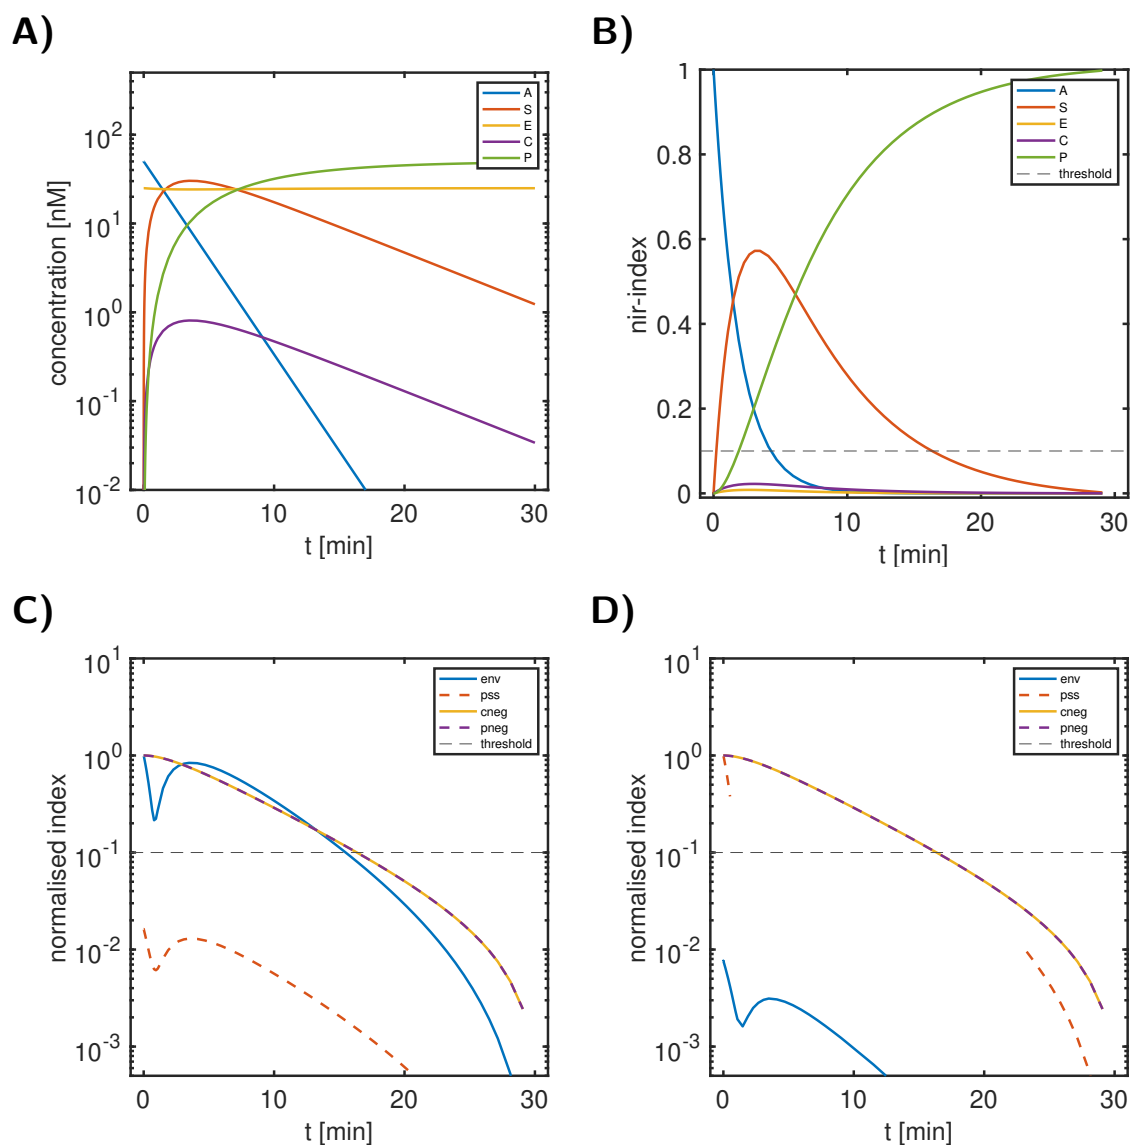

**Figure S9. Scenario 1 of the enzyme kinetics model: time course of state variables and normalised indices . A:** Time course of state variables and **B:** normalized ir-indices. **C:** State classification indices for state C and **D:** for state E.

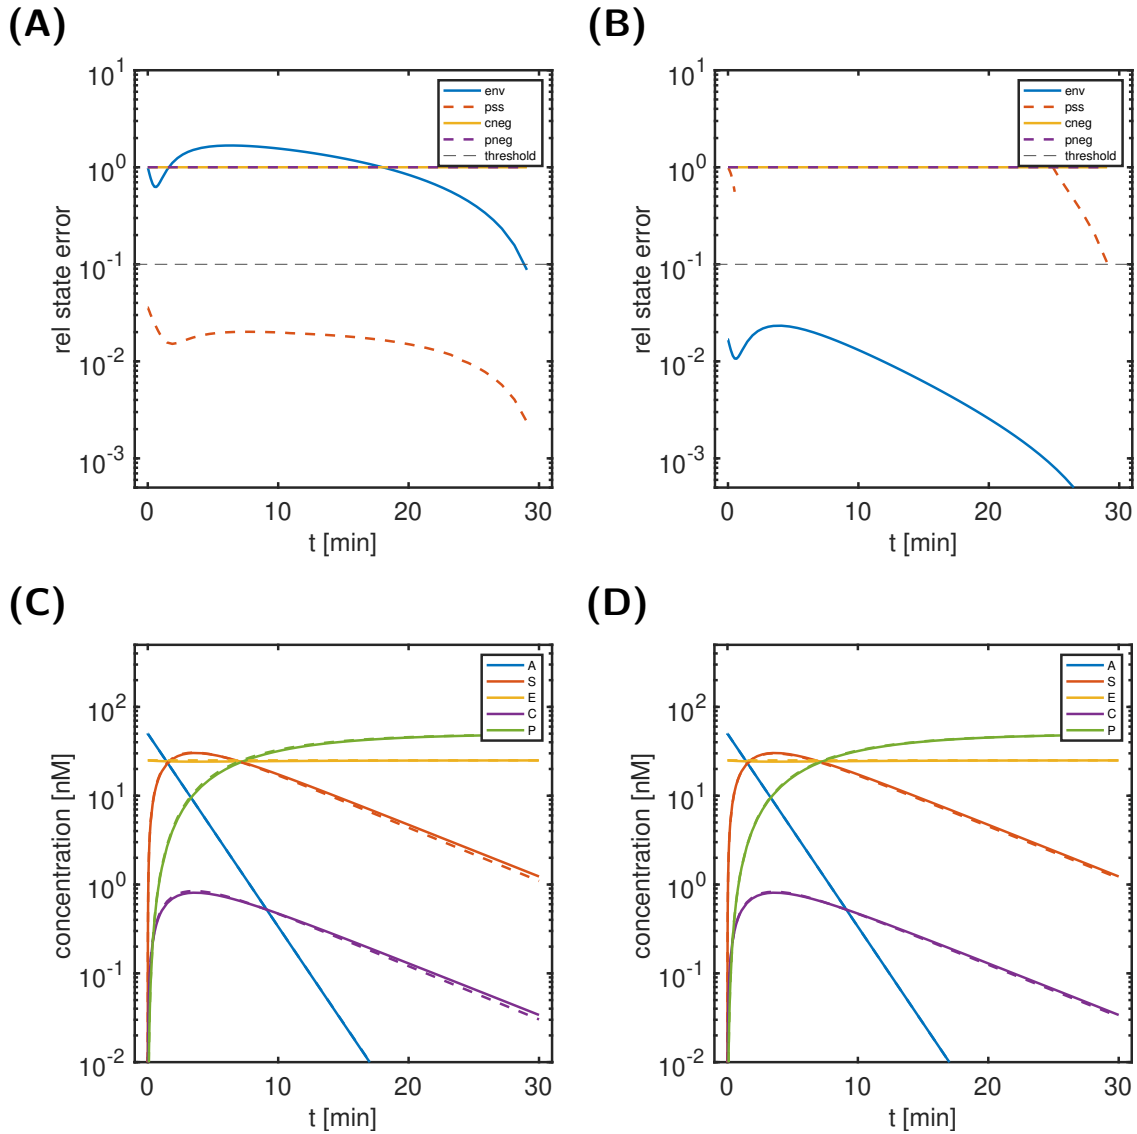

**Figure S10. Scenario 1 of the enzyme kinetics model: Relative state approximation error and modified dynamics .** A: Relative state approximation errors for C and B: for E. C: Comparison of reference dynamics (solid lines) and modified dynamics from  $t^* = 0$  (dashed lines) for C in partial steady state and D: for E as environmental state.

Figure S10 confirms our hypothesized classification. For C (left column) and E (right column), the corresponding relative state approximation errors (top) are below the threshold. A comparison of the reference solution and the solution of the modified system (dashed lines) with C in partial steady state or E environmental, respectively show the very good approximation quality.

The enzyme kinetic example is THE example to illustrate the quasi-steady state or Michaelis-Menten approximation. In its derivation, the conservation of enzyme is typically exploited. In scenario 1, this conservation is not needed to yield good approximation results for the partial steady state approximation of C. In scenario 2, however, the conservation law has to be exploited to obtain high quality approximations. Exploiting a conservation law for E in combination with the partial steady state approximation for C is

identical to first transform the system of ODEs into an equivalent system of ODEs with the equation for  $E$  replaced by  $E_{\text{tot}}$ , i.e., the sum of the equations for  $E$  and  $C$  (i.e., the conserved species). Note that the conservation law still allows to recompute the free enzyme concentration as  $E = E_{\text{tot}} - C$ . Then, the partial steady state approximation for  $C$  can be applied as usual. Transforming a system of ODEs in the described way is nothing else then lumping the states  $E$  and  $C$  into a new state representing  $E_{\text{tot}}$ . In the following, we briefly demonstrate that the indices can be extended to scenarios corresponding to the Michaelis-Menten approximation (scenario 2). An extension of the index analysis approach to conservation laws is, however, beyond the scope of the present article.

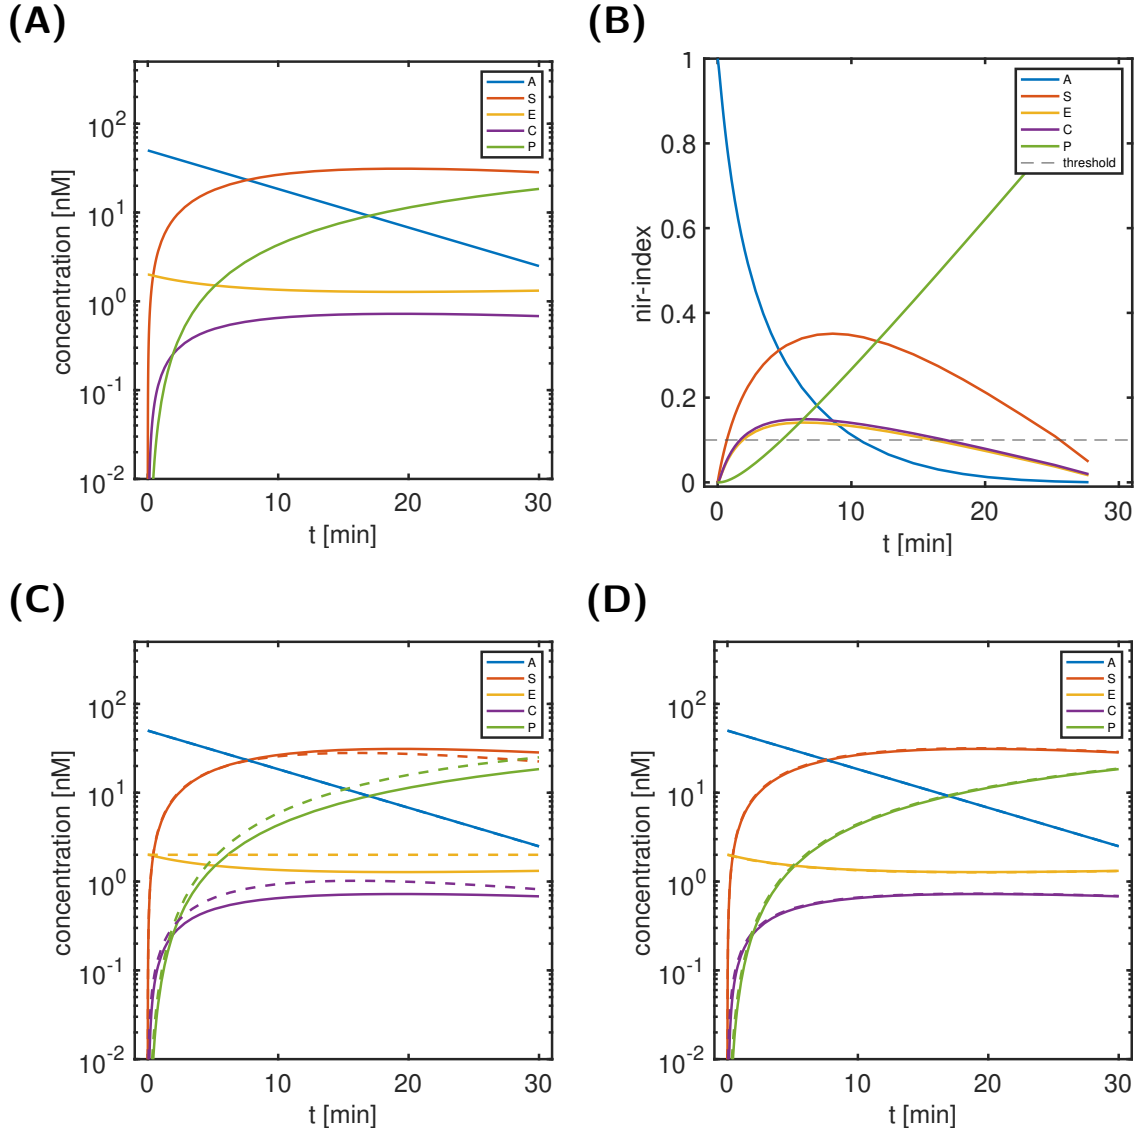

**Figure S11. Scenario 2 of the enzyme kinetic model:** A: Time course of state variables and B: normalised ir-indices. C: Comparison of reference dynamics (solid lines) and modified dynamics from  $t^* = 0$  (dashed lines) for C in partial steady state. D: Comparison of reference dynamics (solid lines) and modified dynamics from  $t^* = 0$  (dashed lines) with conservation law  $E+C = \text{const.}$  in addition to C in partial steady state.

Figure S11A&B shows in the top panel the reference solution (left) and the normalised ir-indices (right) for scenario 2. We infer that all states have to be considered dynamically important. Consequently, assuming C in partial steady state (Figure S11C) results in large approximation errors. In contrast, transforming the system of ODEs as described above allows us to account for the conservation law  $E+C = \text{const.}$  Assuming now C to be in partial steady state yields a very good approximation, as the comparison of reference dynamics (solid lines) and modified dynamics from  $t^* = 0$  (dashed lines) shows (Figure S11D). The resulting approximation is identical to the common Michaelis-Menten approximation for S with  $V_{\max} = 2 \text{ nM/min}$  and  $K_M = 55 \text{ nM}$ .

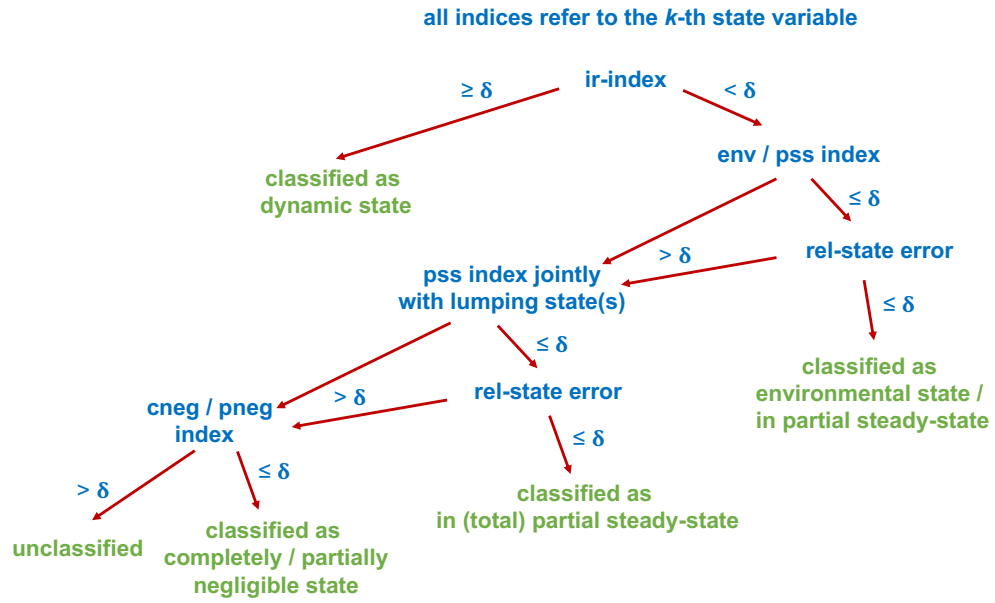

Figure S12. Decision tree for state classification based on indices including lumping

## S5 How to setup a new model for Index Analysis

Setting up a new model is easy and proceeds along the steps below. The `SimpleReactionCycle` folder and files serves as a starting point. The model is described in the first part of the Results in the main manuscript.

Copy the folder `SimpleReactionCycle` and rename it with a meaningful `<ProjectName>`; change into the renamed directory and then into the subfolder `modelspecification`; adapt the following files as outlined below (and rename appropriately by replacing `SimpleReactionCycle_<Filename>.m` with `<YourModelName>_<Filename>.m` )

```
%%% -----
For all template files provided, you only need to adapt the code between the two dashed lines; do not modify
the code outside those line (except for the name of the file in the line starting with function).
%%% -----
```

1. `SimpleReactionCycle_indexing.m`: provide the names of all state variables in the structure `I.nmstate` and the names of all parameters in `I.nmpar`.
2. `SimpleReactionCycle_initialvalues.m`: provide the initial values of the pre-stimulus state of the system; the pre-stimulus state does not include the stimulus (input), which is zero and specified in the `SimpleReactionCycle_model_set_up_details.m`. In the template code, `A` is the stimulus/input and `C` is the output
3. `SimpleReactionCycle_parameters.m`: provide the values for all parameters
4. `SimpleReactionCycle_ode.m`: provide the ordinary differential equations (ODEs);
5. `SimpleReactionCycle_species2params.m`: provide for each state the parameter indices of all reactions that involve that specific state; the information is used for the `cneg` index.
6. `SimpleReactionCycle_model_set_up_details.m`: provides all the final details to simulate the model and compute the indices; provide the model name (i.e. `YourModelName`, see above), specify the input state, the output state and the simulation time span; in addition, you can specify different scenarios (in the template code, different values for a parameter); if a jacobian or legend labels are provided (see below), set corresponding binary variables to `true`.
7. `SimpleReactionCycle_odejac.m` (optional): provide the jacobian of the system of ODEs; if no jacobian is provided then the ODE solver uses a standard numerical approximation. Note: errors in jacobians for larger systems are easily made, in particular, if it is a larger system and done manually; do compare your results with the case, where the jacobian is numerically determined by MATLAB.
8. `SimpleReactionCycle_legendlabels.m` (optional): sometimes the names in the code are not easily readable when used in a figure legend; here one can provide for each state a name used in figure legend.

Finally, exit the directory `modelspecification` to the parent `<ProjectName>` directory. The final step is to adapt the main script `SimpleReactionCycle_MAIN.m` (rename meaningfully to `<YourModelName>_MAIN.m`). Specify the model name and the scenario (see `SimpleReactionCycle_model_set_up_details.m` above) and the desired analysis plots.

You are now ready to run the main script `<YourModelName>_MAIN.m` !

## S6 Additional figures and tables for in the index analysis of the EGFR system

### A) membrane EGFR signalling

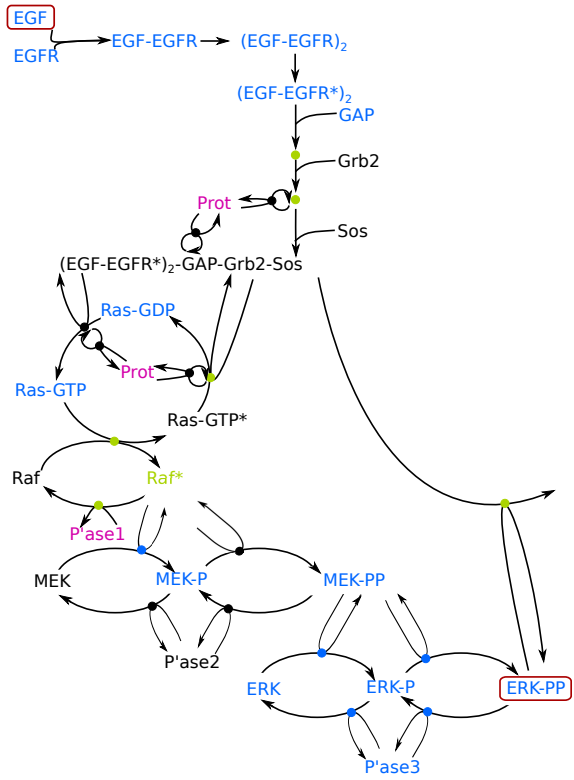

### B) internalised EGFR signalling

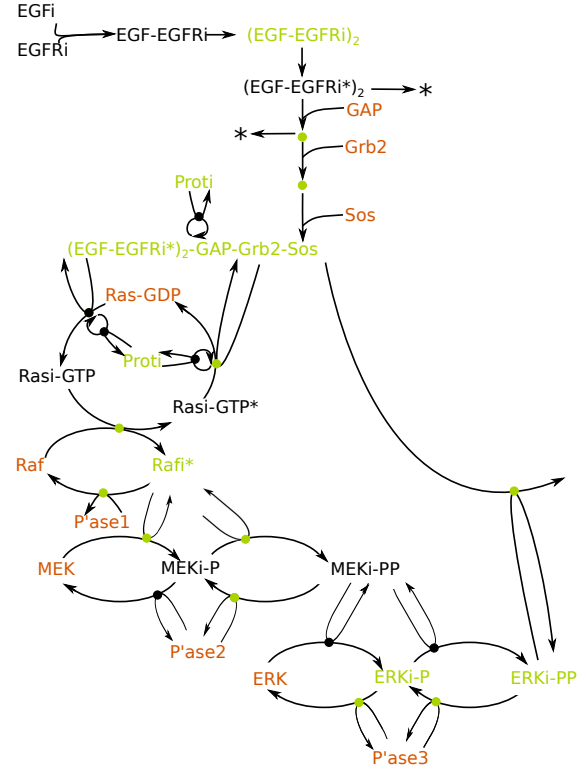

**Figure S13. Schematic with state classification of the signal transduction network focussing on the Shc-independent pathway**, including the state variables with large maximum input-response index (light blue, see Figure 4D), environmental state variables (purple), state variables in partial-steady state (green) and further state variables (dark blue). States being part of the membrane-bound and internalised pathway are coloured orange in panel (B). The red boxes mark the input and output state variables. Note that the difference to the Shc-dependent pathway is the absence of Shc (adaptor protein between GAP and Grb2).

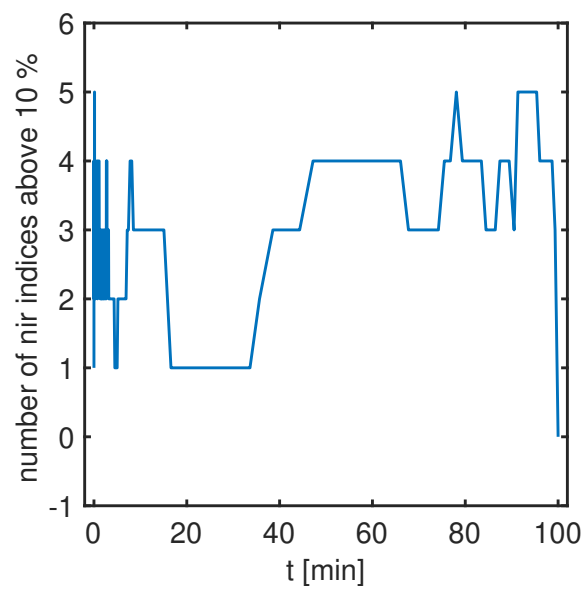

Figure S14. Number of normalised ir-indices above the threshold of 10% as a function of time.

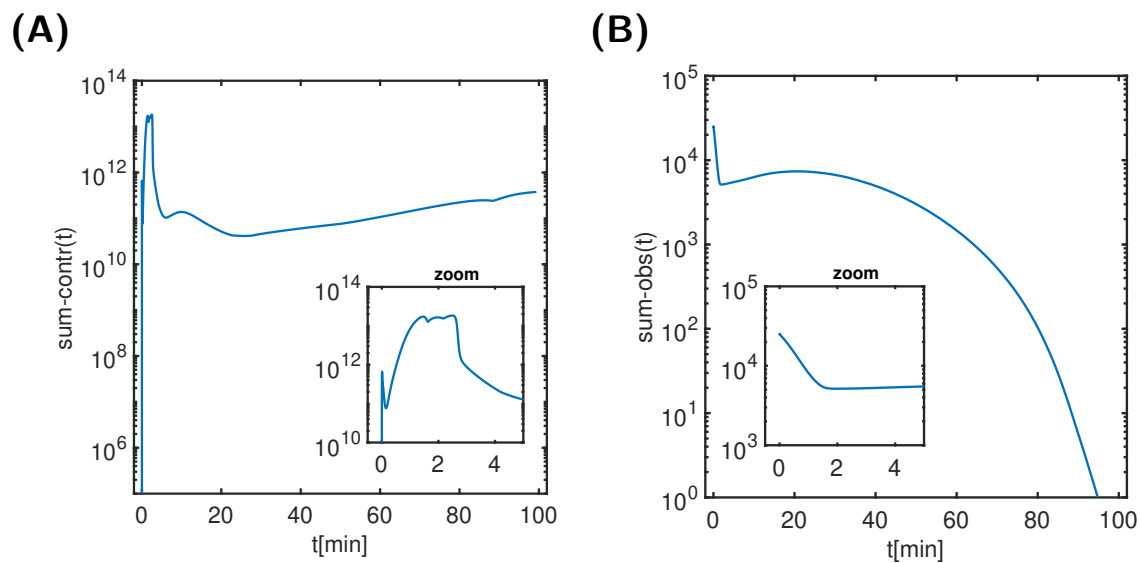

**Figure S15. Sum of contr- and obs-indices evolving over time.** Left: Sum of contr-indices over time, showing three phases: initial sharp peak (0-0.3 min), second prolonged peak (0.3-3 min), and a slow, still incomplete recovery period (3-100 min). Right: Sum of obs-indices over time, showing three phases: initial sharp decline (0-1.5 min), marginal increase (1.5-20 min), and a strong decline (20-100 min). Note the very different scales on the y-axis.

**Table S3. Normalised input-response indices for the EGFR system; sorted according to their maximum**

| No. | Variable name                                            | max(nir-index) |
|-----|----------------------------------------------------------|----------------|
| 1   | EGF                                                      | 1              |
| 2   | EGFR                                                     | 4.95e-01       |
| 3   | EGF-EGFR                                                 | 4.76e-01       |
| 4   | (EGF-EGFR*) <sub>2</sub>                                 | 4.57e-01       |
| 5   | MEK-P                                                    | 4.37e-01       |
| 6   | ERK-P-MEK-PP                                             | 3.78e-01       |
| 7   | ERK-PP                                                   | 3.44e-01       |
| 8   | Phosphatase3                                             | 3.23e-01       |
| 9   | Ras-GDP                                                  | 3.10e-01       |
| 10  | ERK-P                                                    | 2.89e-01       |
| 11  | ERK                                                      | 2.83e-01       |
| 12  | ERK-MEK-PP                                               | 2.78e-01       |
| 13  | (EGF-EGFR) <sub>2</sub>                                  | 2.43e-01       |
| 14  | ERK-P-P'ase3                                             | 1.99e-01       |
| 15  | Ras-GTP                                                  | 1.99e-01       |
| 16  | ERK-PP-P'ase3                                            | 1.72e-01       |
| 17  | GAP                                                      | 1.66e-01       |
| 18  | MEK-Raf*                                                 | 1.56e-01       |
| 19  | MEK-PP                                                   | 1.48e-01       |
| 20  | (EGF-EGFR*) <sub>2</sub> -GAP-Shc*-Grb2-Sos-Ras-GDP      | 1.32e-01       |
| 21  | (EGF-EGFR*) <sub>2</sub> -GAP-Shc*-Grb2-Sos              | 9.90e-02       |
| 22  | ERKi-P                                                   | 5.44e-02       |
| 23  | MEK-P-Raf*                                               | 4.64e-02       |
| 24  | MEK                                                      | 3.64e-02       |
| 25  | ERKi-P-P'ase3i                                           | 3.10e-02       |
| 26  | Ras-GTP*                                                 | 3.00e-02       |
| 27  | ERKi-PP                                                  | 2.88e-02       |
| 28  | Shc*                                                     | 2.80e-02       |
| 29  | Shc                                                      | 2.66e-02       |
| 30  | (EGF-EGFR*) <sub>2</sub> -GAP-Shc*-Grb2-Sos-ERK-PP       | 2.38e-02       |
| 31  | ERKi-PP-P'ase3i                                          | 2.09e-02       |
| 32  | Raf                                                      | 2.05e-02       |
| 33  | (EGF-EGFR*) <sub>2</sub> -GAP-Shc*-Grb2-Sos-Prot         | 1.97e-02       |
| 34  | MEKi-PP                                                  | 1.76e-02       |
| 35  | (EGF-EGFR*) <sub>2</sub> -GAP-Grb2-Sos-Ras-GDP           | 1.72e-02       |
| 36  | (EGF-EGFRi*) <sub>2</sub> -GAP-Shc*-Grb2-Sos             | 1.66e-02       |
| 37  | Phosphatase2                                             | 1.53e-02       |
| 38  | (EGF-EGFR*) <sub>2</sub> -GAP-Shc*                       | 1.53e-02       |
| 39  | Grb2-Sos                                                 | 1.47e-02       |
| 40  | (EGF-EGFR*) <sub>2</sub> -GAP-Shc*-Grb2-Sos-Ras-GTP      | 1.38e-02       |
| 41  | (EGF-EGFR*) <sub>2</sub> -GAP-Grb2-Sos                   | 1.27e-02       |
| 42  | Rasi-GTP*                                                | 1.26e-02       |
| 43  | Raf-Ras-GTP                                              | 1.25e-02       |
| 44  | ERKi-P-MEKi-PP                                           | 1.05e-02       |
| 45  | ERKi-MEKi-PP                                             | 1.05e-02       |
| 46  | (EGF-EGFR*) <sub>2</sub> -GAP-Shc*-Grb2-Sos-Ras-GDP-Prot | 9.92e-03       |
| 47  | (EGF-EGFR*) <sub>2</sub> -GAP                            | 9.83e-03       |

*Table is continued on next page*

Table S3 – cont.

| No. | Variable name                                            | max(nir-index) |
|-----|----------------------------------------------------------|----------------|
| 48  | Prot                                                     | 9.66e-03       |
| 49  | (EGF-EGFR*) <sub>2</sub> -GAP-Shc*-Grb2-Sos-Ras-GTP-Prot | 9.30e-03       |
| 50  | MEK-PP-Pase2                                             | 9.05e-03       |
| 51  | (EGF-EGFRi*) <sub>2</sub> -GAP-Shc*                      | 8.01e-03       |
| 52  | Phosphatase1                                             | 7.86e-03       |
| 53  | Raf*-Pase                                                | 6.81e-03       |
| 54  | (EGF-EGFRi*) <sub>2</sub>                                | 6.57e-03       |
| 55  | MEKi-Rafi*                                               | 6.34e-03       |
| 56  | (EGF-EGFR*) <sub>2</sub> -GAP-Shc                        | 6.00e-03       |
| 57  | MEKi-P                                                   | 5.76e-03       |
| 58  | (EGF-EGFRi*) <sub>2</sub> -GAP-Shc*-Grb2-Sos-Ras-GDP     | 5.10e-03       |
| 59  | Shc*-Grb2-Sos                                            | 4.85e-03       |
| 60  | (EGF-EGFR*) <sub>2</sub> -GAP-Grb2-Sos-ERK-PP            | 4.04e-03       |
| 61  | (EGF-EGFRi*) <sub>2</sub> -GAP                           | 3.78e-03       |
| 62  | MEKi-PP-Pase2i                                           | 2.71e-03       |
| 63  | (EGF-EGFR*) <sub>2</sub> -GAP-Grb2-Sos-Ras-GTP           | 2.51e-03       |
| 64  | MEKi-P-Pase2i                                            | 2.37e-03       |
| 65  | (EGF-EGFRi*) <sub>2</sub> -GAP-Grb2-Sos                  | 2.35e-03       |
| 66  | (EGF-EGFR*) <sub>2</sub> -GAP-Shc*-Grb2                  | 2.28e-03       |
| 67  | MEK-P-Pase2                                              | 2.17e-03       |
| 68  | (EGF-EGFRi*) <sub>2</sub> -GAP-Shc*-Grb2-Sos-Ras-GTP     | 2.16e-03       |
| 69  | (EGF-EGFR*) <sub>2</sub> -GAP-Grb2                       | 2.02e-03       |
| 70  | (EGF-EGFR*) <sub>2</sub> -GAP-Grb2-Sos-Prot              | 1.92e-03       |
| 71  | Grb2                                                     | 1.83e-03       |
| 72  | Rasi-GTP                                                 | 1.80e-03       |
| 73  | Raf*                                                     | 1.73e-03       |
| 74  | (EGF-EGFR*) <sub>2</sub> -GAP-Grb2-Sos-Ras-GDP-Prot      | 1.38e-03       |
| 75  | EGFRi                                                    | 1.22e-03       |
| 76  | Rafi*-Pase                                               | 1.16e-03       |
| 77  | (EGF-EGFR*) <sub>2</sub> -GAP-Grb2-Sos-Ras-GTP-Prot      | 1.06e-03       |
| 78  | EGF-EGFRi                                                | 1.01e-03       |
| 79  | (EGF-EGFRi*) <sub>2</sub> -GAP-Grb2-Sos-Ras-GDP          | 9.57e-04       |
| 80  | Sos-ERK-PP                                               | 8.99e-04       |
| 81  | Shc*-Grb2                                                | 7.28e-04       |
| 82  | (EGF-EGFRi*) <sub>2</sub> -GAP-Shc                       | 7.25e-04       |
| 83  | (EGF-EGFRi*) <sub>2</sub> -GAP-Shc*-Grb2                 | 7.22e-04       |
| 84  | (EGF-EGFR*) <sub>2</sub> -GAP-Grb2-Prot                  | 5.75e-04       |
| 85  | (EGF-EGFRi*) <sub>2</sub> -GAP-Grb2                      | 5.48e-04       |
| 86  | (EGF-EGFR*) <sub>2</sub> -GAP-Shc*-Grb2-Prot             | 5.40e-04       |
| 87  | Sos                                                      | 5.25e-04       |
| 88  | EGFi                                                     | 4.86e-04       |
| 89  | MEKi-P-Rafi*                                             | 4.12e-04       |
| 90  | (EGF-EGFRi*) <sub>2</sub> -GAP-Grb2-Sos-Ras-GTP          | 2.67e-04       |
| 91  | (EGF-EGFRi*) <sub>2</sub> -GAP-Shc*-Grb2-Sos-ERKi-PP     | 2.67e-04       |
| 92  | Sos-ERKi-PP                                              | 1.20e-04       |
| 93  | Rafi-Rasi-GTP                                            | 1.01e-04       |
| 94  | Rafi*                                                    | 7.31e-05       |
| 95  | (EGF-EGFRi) <sub>2</sub>                                 | 5.94e-05       |

Table is continued on next page

Table S3 – cont.

| No. | Variable name                                                   | max(nir-index) |
|-----|-----------------------------------------------------------------|----------------|
| 96  | (EGF-EGFRi*) <sub>2</sub> -GAP-Grb2-Sos-ERKi-PP                 | 5.44e-05       |
| 97  | Proti                                                           | 1.41e-08       |
| 98  | (EGF-EGFRi*) <sub>2</sub> -GAP-Shc <sub>deg</sub>               | 0              |
| 99  | (EGF-EGFRi*) <sub>2</sub> -GAP <sub>deg</sub>                   | 0              |
| 100 | (EGF-EGFRi*) <sub>2</sub> -GAP-Grb2-Sos-Ras <sub>deg</sub>      | 0              |
| 101 | (EGF-EGFRi*) <sub>2</sub> -GAP-Shc*-Grb2-Sos-Ras <sub>deg</sub> | 0              |
| 102 | AUC ERK-PP                                                      | 0              |
| 103 | Sosi                                                            | 0              |
| 104 | (EGF-EGFRi*) <sub>2</sub> -GAP-Shc*-Grb2-Sos <sub>deg</sub>     | 0              |
| 105 | (EGF-EGFRi*) <sub>2</sub> -GAP-Grb2 <sub>deg</sub>              | 0              |
| 106 | (EGF-EGFRi*) <sub>2</sub> -GAP-Grb2-Sos <sub>deg</sub>          | 0              |
| 107 | (EGF-EGFR*) <sub>2</sub> -GAP-Shc*-Grb2-Sos <sub>deg</sub>      | 0              |
| 108 | (EGF-EGFRi*) <sub>2</sub> -GAP-Shc*-Grb2 <sub>deg</sub>         | 0              |
| 109 | (EGF-EGFR*) <sub>2</sub> -GAP-Grb2-Sos <sub>deg</sub>           | 0              |
| 110 | (EGF-EGFRi*) <sub>2deg</sub>                                    | 0              |
| 111 | EGFRi <sub>deg</sub>                                            | 0              |
| 112 | EGFi <sub>deg</sub>                                             | 0              |

## References

1. Deuffhard P, Bornemann F. Scientific Computing with Ordinary Differential Equations. Springer, New York, 2002, 1st ed.
